# Supplementary material for: Koopmans-compliant functionals and their performance against reference molecular data
Source: arXiv:1405.4635 source file (2014-08-19)
Supplement: Supplementary file 1 [file Supplemental_Material.pdf]

# Koopmans-compliant functionals and their performance against reference molecular data: supplemental material

Giovanni Borghi,[1,*] Andrea Ferretti,[2] Linh Nguyen,[1] Ismaila Dabo,[3] and Nicola Marzari[1]

[1] *Theory and Simulations of Materials (THEOS), and National Center for Computational Design and Discovery of Novel Materials (MARVEL), École Polytechnique Fédérale de Lausanne, 1015 Lausanne, Switzerland*

[2] *Centro S3, CNR–Istituto Nanoscienze, I-41125 Modena, Italy*

[3] *Department of Materials Science and Engineering, Materials Research Institute, and Penn State Institutes of Energy and the Environment, The Pennsylvania State University, University Park, PA 16802, USA*

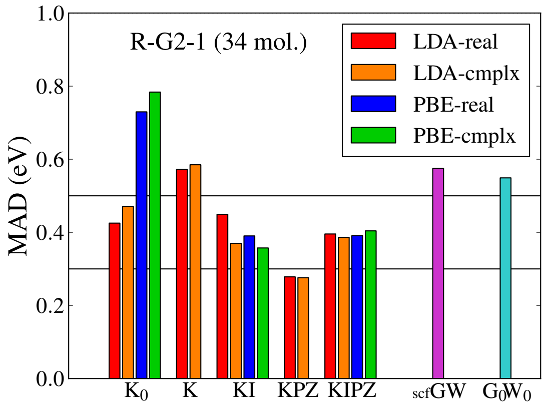


Figure 1. Enlarged view of Fig. 2 (b) in the paper.

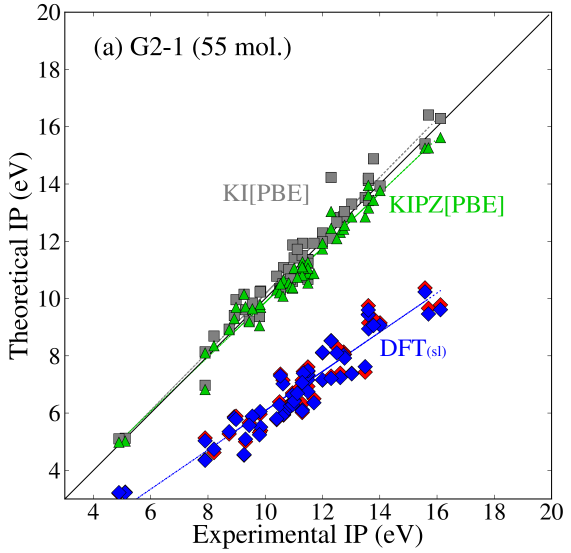


Figure 2. Theoretical vs. experimental ionization energies for the full 55 molecule G2-1 set (see also Fig. 3 in the paper) and for KI and KIPZ computed on top of PBE and with complex wavefunctions. Dashed lines are linear fits of theoretical data.

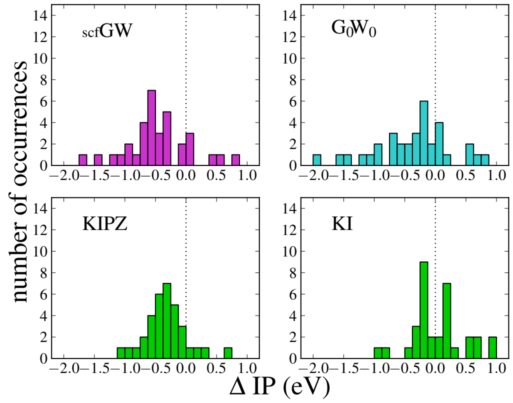


Figure 3. Distribution of mismatches between theoretical and experimental ionization energy for the 34 R-G2-1 molecules. The color of the bars is coherent to the legend of Fig. 2 (b) in the paper, telling on top of what type of functional the Koopmans' correction has been applied, and whether real or complex wavefunctions have been used. In this case KI and KIPZ results were obtained on top of PBE and with complex wavefunctions.

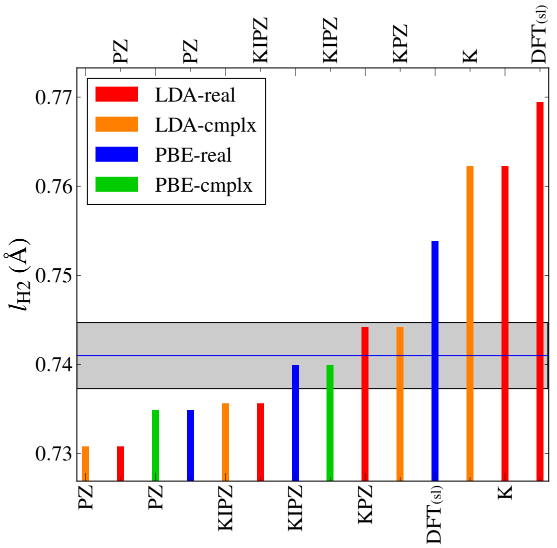


Figure 4. $H_2$ bond length computed with LDA, PBE, PZ and all variational flavors of Koopmans-compliant functionals. The shaded region marks the range of bond lengths which deviate less than 0.5% from the experimental value. The KIPZ functional on top of PBE and minimized on the space of complex wavefunctions succesfully interpolates between the Perdew-Zunger and the PBE predictions, finding a bond length in very good agreement with experiment.

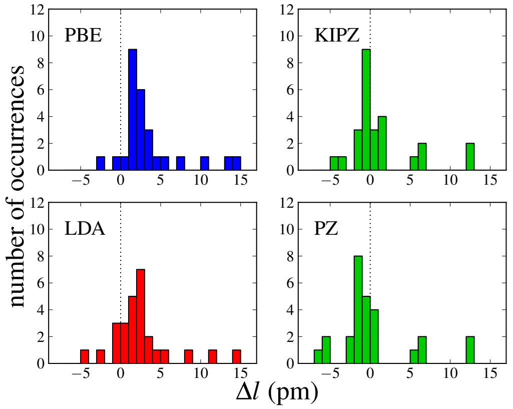


Figure 5. The $y$ axes of the four above panels show the number of dimers in the G2-1 set whose experimental bond-length prediction deviates from experiment by a quantity specified (in picometers) by the $x$ coordinate. The dimers in this test-set are listed in the caption of Fig. 4 of the paper. The PZ and KIPZ functionals shown above have been minimized on the set of complex wavefunctions. The color of the bars is coherent to the legend of Fig. 2 in the paper, and tells the base functional on top of which the Koopmans' correction has been applied, and whether real or complex wavefunctions have been used. In this case KIPZ and PZ results were computed on top of PBE and with complex wavefunctions. Note how both LDA and PBE overestimate bond lengths systematically, while the distribution of deviations of KIPZ is approximately centered around zero error.

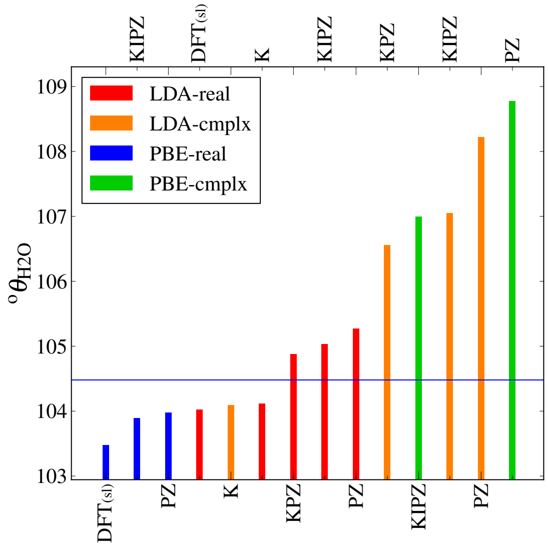


Figure 6. $H_2O$ (HOH) angle (in degrees) computed with LDA, PBE, PZ and all variational flavors of Koopmans-compliant functionals. Apart from the K Koopmans flavor, all other ODD schemes are equivalent to or less accurate than LDA or PBE. KC schemes generally improve over the PZ-SIC scheme on top of the same base functional.

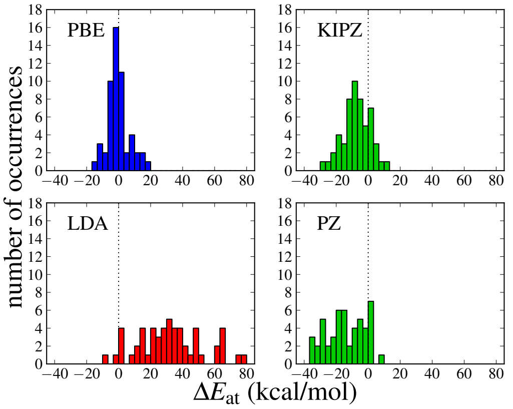


Figure 7. Distribution of deviations of atomization energies of G2-1 set molecules (plus $H_2$) from experiment. The bottom-left panel shows the severe over-estimation of atomization energies within the Local Density Approximation. The KIPZ functional on top of PBE shows a systematic under-estimation of around 10 kcal/mol, which, is slightly smaller than that displayed by the PZ functional. The color of the bars is coherent to the legend of Fig. 2 in the paper, and tells on top of what type of functional the Koopmans' correction has been applied, and whether real or complex wavefunctions have been used. In this case KIPZ and PZ results were computed on top of PBE and with complex wavefunctions.

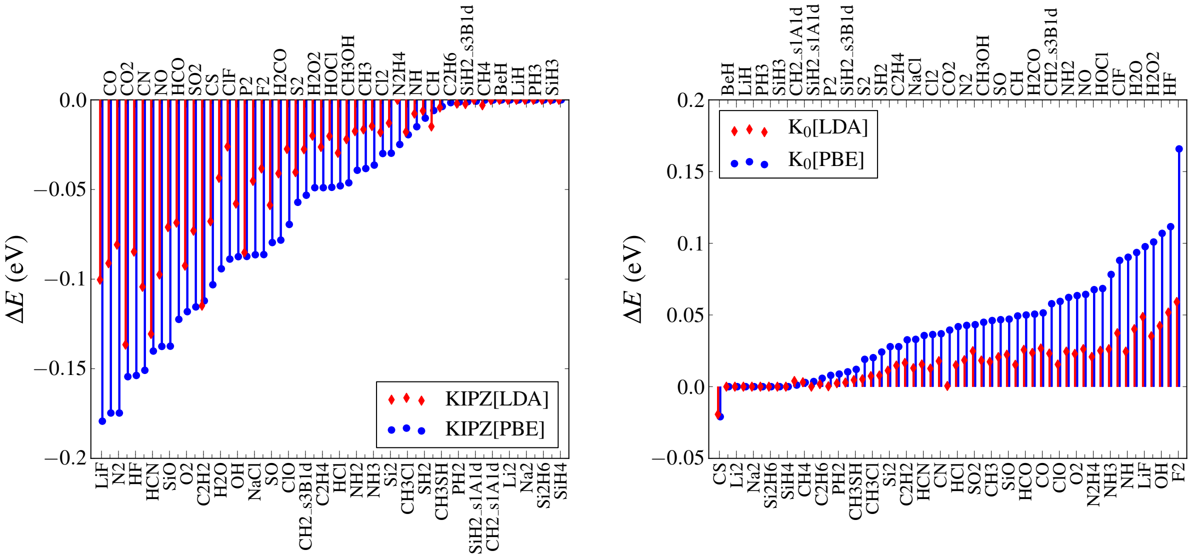


Figure 8. Left panel: energy difference per electron (in eV) between the complex-valued and the real-valued wavefunction minimum for the KIPZ functional. The red bars show the result for the LDA functional, while the blue bars show the same for PBE. The energy gain is maximum for $CO_2$ and absent in alkaline dimers and Silicon and Carbon sp3 compounds. Right panel: same energy difference for the non-variational $K_0$ functional. Molecules have been arranged in order of increasing PBE energy difference.

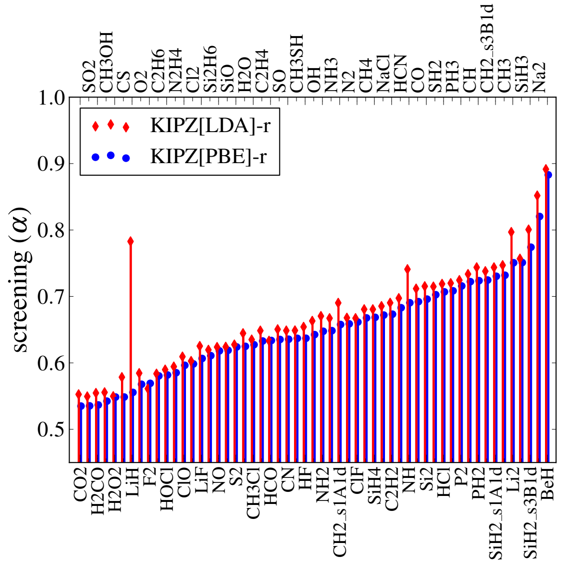


Figure 9. Screening coefficients for all molecules in the G2-1 set, whose ground-state energy has been computed with the KIPZ functional and minimized on the space of real wavefunctions.

| | exp | LDA | PZ | KI | KIPZ | $K_0$ | K | KPZ |
|---|---|---|---|---|---|---|---|---|
| LiH | 7.90 | 4.37 | 8.74 | 8.11 | 8.14 | 7.64 | 7.47 | 7.34 |
| BeH | 8.21 | 4.62 | 8.76 | 8.56 | 8.55 | 8.44 | 8.34 | 8.25 |
| CH | 10.64 | 5.93 | 12.16 | 10.97 | 11.12 | 10.50 | 10.99 | 10.58 |
| $CH_2$_s3B1d | 10.40 | 5.77 | 11.55 | 11.00 | 10.77 | 10.11 | 10.83 | 10.38 |
| $CH_3$ | 9.84 | 5.39 | 10.46 | 9.92 | 9.97 | 9.34 | 9.96 | 9.61 |
| $CH_4$ | 13.60 | 9.45 | 15.95 | 14.23 | 14.52 | 13.85 | 14.46 | 14.15 |
| NH | 13.49 | 7.43 | 14.70 | 13.57 | 13.59 | 12.58 | 13.68 | 13.14 |
| $NH_2$ | 12.00 | 7.15 | 13.89 | 12.32 | 12.33 | 11.39 | 12.16 | 11.79 |
| $NH_3$ | 10.82 | 6.27 | 12.59 | 11.37 | 11.29 | 10.32 | 11.32 | 10.89 |
| OH | 13.02 | 7.39 | 15.37 | 13.67 | 13.50 | 12.31 | 13.43 | 12.87 |
| $H_2O$ | 12.62 | 7.39 | 14.81 | 13.26 | 13.13 | 11.91 | 13.35 | 12.73 |
| HF | 16.12 | 9.78 | 18.49 | 16.83 | 16.66 | 15.15 | 16.93 | 16.18 |
| $SiH_2$_s1A1d | 8.92 | 5.87 | 10.26 | 9.85 | 9.71 | 9.35 | 9.68 | 9.35 |
| $SiH_3$ | 8.74 | 5.27 | 9.83 | 9.16 | 9.20 | 8.90 | 9.18 | 8.94 |
| $SiH_4$ | 12.30 | 8.53 | 14.20 | 12.39 | 12.87 | 12.47 | 12.71 | 12.55 |
| $PH_2$ | 9.82 | 5.96 | 10.78 | 10.48 | 10.22 | 9.76 | 10.28 | 9.95 |
| $PH_3$ | 10.95 | 6.70 | 11.55 | 10.60 | 10.85 | 10.34 | 10.92 | 10.44 |
| $SH_2$ | 10.50 | 6.39 | 11.50 | 10.71 | 10.83 | 10.16 | 10.89 | 10.54 |
| HCl | 12.74 | 8.13 | 13.83 | 12.92 | 13.16 | 12.32 | 12.39 | 11.92 |
| $Li_2$ | 5.11 | 3.24 | 5.42 | 5.30 | 5.27 | 5.02 | 4.97 | 4.86 |
| LiF | 11.30 | 6.32 | 13.81 | 12.32 | 12.09 | 10.60 | 12.61 | 11.70 |
| $C_2H_2$ | 11.49 | 7.33 | 12.60 | 11.70 | 11.85 | 11.04 | 12.04 | 11.53 |
| $C_2H_4$ | 11.49 | 6.93 | 12.27 | 10.92 | 11.21 | 10.41 | 11.37 | 10.90 |
| $C_2H_6$ | 12.00 | 8.10 | 14.58 | 12.13 | 12.42 | 12.13 | 12.62 | 12.20 |
| CN | 13.60 | 9.75 | 15.59 | 14.43 | 14.43 | 13.40 | 14.48 | 14.15 |
| HCN | 13.61 | 9.15 | 14.89 | 13.80 | 14.17 | 13.25 | 14.32 | 13.83 |
| CO | 14.01 | 9.15 | 15.68 | 14.30 | 14.51 | 13.77 | 14.19 | 14.18 |
| HCO | 9.31 | 5.00 | 12.18 | 9.80 | 10.20 | 9.76 | 10.37 | 9.95 |
| $H_2CO$ | 10.88 | 6.34 | 13.77 | 12.28 | 11.17 | 10.38 | 11.65 | 10.83 |
| $CH_3OH$ | 10.96 | 6.39 | 13.62 | 11.26 | 11.14 | 10.33 | 11.61 | 10.84 |
| $N_2$ | 15.58 | 10.37 | 17.75 | 16.34 | 16.16 | 15.48 | 16.20 | 15.89 |
| $N_2H_4$ | 8.98 | 5.89 | 12.40 | 10.68 | 10.47 | 9.70 | 10.78 | 10.22 |
| NO | 9.26 | 4.53 | 12.94 | 10.84 | 10.59 | 9.93 | 10.84 | 10.29 |
| $O_2$ | 12.30 | 7.29 | 16.30 | 12.81 | 13.48 | 12.59 | 14.04 | 13.16 |
| $H_2O_2$ | 11.70 | 6.50 | 14.42 | 12.31 | 11.65 | 10.93 | 12.28 | 11.44 |
| $F_2$ | 15.70 | 9.66 | 19.17 | 16.54 | 15.99 | 15.19 | 16.75 | 15.72 |
| $CO_2$ | 13.78 | 9.30 | 16.32 | 14.69 | 14.01 | 13.33 | 14.77 | 13.78 |
| $Na_2$ | 4.89 | 3.19 | 5.11 | 5.17 | 5.13 | 4.97 | 4.87 | 4.75 |
| $Si_2$ | 7.90 | 5.13 | 9.03 | 8.53 | 8.52 | 8.18 | 8.68 | 8.31 |
| $P_2$ | 10.62 | 7.15 | 11.02 | 10.70 | 10.75 | 10.18 | 10.87 | 10.54 |
| $S_2$ | 9.55 | 5.88 | 11.34 | 9.75 | 10.00 | 9.64 | 11.05 | 10.92 |
| $Cl_2$ | 11.49 | 7.45 | 13.32 | 11.76 | 11.76 | 11.28 | 12.64 | 11.07 |
| NaCl | 9.80 | 5.32 | 10.28 | 9.63 | 9.58 | 8.64 | 9.67 | 8.82 |
| SiO | 11.49 | 7.61 | 12.94 | 12.08 | 11.66 | 11.18 | 12.08 | 11.46 |
| CS | 11.33 | 7.45 | 13.48 | 11.21 | 11.56 | 10.87 | 11.60 | 11.37 |
| SO | 11.29 | 6.02 | 12.72 | 10.81 | 11.15 | 10.66 | 11.38 | 10.81 |
| ClO | 11.01 | 6.45 | 13.63 | 11.95 | 11.78 | 11.26 | 12.00 | 11.26 |
| ClF | 12.77 | 8.05 | 14.55 | 12.57 | 13.32 | 12.72 | 12.88 | 12.38 |
| $Si_2H_6$ | 10.53 | 7.36 | 12.28 | 10.30 | 10.92 | 10.58 | 10.97 | 10.68 |
| $CH_3Cl$ | 11.29 | 7.15 | 12.94 | 11.03 | 11.62 | 10.98 | 11.72 | 11.03 |
| $CH_3SH$ | 9.44 | 5.66 | 10.90 | 9.79 | 9.77 | 9.22 | 9.91 | 9.52 |
| HOCl | 11.12 | 6.81 | 13.33 | 11.23 | 11.49 | 10.93 | 11.84 | 11.08 |
| $SO_2$ | 12.50 | 8.30 | 15.22 | 12.55 | 12.86 | 12.35 | 13.39 | 12.71 |

Table I. Tabulated ionization energies (in eV) for all molecules of the G2-1 set and for all functionals discussed in the paper having LDA as base functional, and being minimized on the set of real wavefunctions.

| | exp | LDA | PZ | KI | KIPZ | $K_0$ | K | KPZ |
|---|---|---|---|---|---|---|---|---|
| LiH | 7.90 | 4.37 | 8.74 | 8.11 | 8.14 | 7.64 | 7.47 | 7.34 |
| BeH | 8.21 | 4.62 | 8.76 | 8.56 | 8.55 | 8.44 | 8.34 | 8.25 |
| CH | 10.64 | 5.93 | 12.07 | 11.25 | 11.25 | 10.49 | 11.00 | 10.69 |
| $CH_2$_s3B1d | 10.40 | 5.77 | 11.15 | 10.87 | 10.72 | 10.09 | 10.82 | 10.33 |
| $CH_3$ | 9.84 | 5.39 | 10.14 | 10.25 | 9.95 | 9.30 | 9.91 | 9.57 |
| $CH_4$ | 13.60 | 9.45 | 15.93 | 14.29 | 14.54 | 13.85 | 14.46 | 14.18 |
| NH | 13.49 | 7.43 | 14.55 | 13.80 | 13.57 | 12.58 | 13.69 | 13.19 |
| $NH_2$ | 12.00 | 7.15 | 13.84 | 12.51 | 12.32 | 11.39 | 12.16 | 11.80 |
| $NH_3$ | 10.82 | 6.27 | 12.40 | 11.35 | 11.26 | 10.32 | 11.32 | 10.89 |
| OH | 13.02 | 7.39 | 15.20 | 13.60 | 13.68 | 12.30 | 13.43 | 13.05 |
| $H_2O$ | 12.62 | 7.39 | 14.41 | 13.26 | 13.06 | 11.90 | 13.35 | 12.66 |
| HF | 16.12 | 9.78 | 18.10 | 16.77 | 16.80 | 15.12 | 16.92 | 16.30 |
| $SiH_2$_s1A1d | 8.92 | 5.87 | 10.26 | 9.58 | 9.71 | 9.35 | 9.68 | 9.35 |
| $SiH_3$ | 8.74 | 5.27 | 9.83 | 8.93 | 9.20 | 8.90 | 9.17 | 8.94 |
| $SiH_4$ | 12.30 | 8.53 | 14.20 | 12.15 | 12.87 | 12.47 | 12.71 | 12.55 |
| $PH_2$ | 9.82 | 5.96 | 10.71 | 10.26 | 10.20 | 9.76 | 10.28 | 9.94 |
| $PH_3$ | 10.95 | 6.70 | 11.54 | 10.79 | 10.85 | 10.34 | 10.94 | 10.44 |
| $SH_2$ | 10.50 | 6.39 | 11.39 | 10.65 | 10.81 | 10.16 | 10.93 | 10.53 |
| HCl | 12.74 | 8.13 | 13.58 | 13.18 | 13.20 | 12.32 | 12.82 | 12.23 |
| $Li_2$ | 5.11 | 3.24 | 5.42 | 5.30 | 5.27 | 5.02 | 4.97 | 4.86 |
| LiF | 11.30 | 6.32 | 13.67 | 12.54 | 12.32 | 10.57 | 12.60 | 11.93 |
| $C_2H_2$ | 11.49 | 7.33 | 11.45 | 11.77 | 11.66 | 10.69 | 11.98 | 11.27 |
| $C_2H_4$ | 11.49 | 6.93 | 11.89 | 11.06 | 11.16 | 10.38 | 11.37 | 10.86 |
| $C_2H_6$ | 12.00 | 8.10 | 14.56 | 11.98 | 12.35 | 12.15 | 12.62 | 12.18 |
| CN | 13.60 | 9.75 | 14.50 | 14.82 | 14.14 | 13.08 | 14.55 | 13.89 |
| HCN | 13.61 | 9.15 | 13.81 | 13.82 | 14.03 | 12.91 | 14.35 | 13.70 |
| CO | 14.01 | 9.15 | 15.76 | 14.25 | 14.50 | 13.81 | 14.17 | 14.22 |
| HCO | 9.31 | 5.00 | 12.07 | 9.58 | 10.19 | 9.76 | 10.37 | 9.96 |
| $H_2CO$ | 10.88 | 6.34 | 13.51 | 11.18 | 11.15 | 10.38 | 11.65 | 10.86 |
| $CH_3OH$ | 10.96 | 6.39 | 13.29 | 11.73 | 11.09 | 10.31 | 11.62 | 10.79 |
| $N_2$ | 15.58 | 10.37 | 16.86 | 15.72 | 16.05 | 15.48 | 16.19 | 15.81 |
| $N_2H_4$ | 8.98 | 5.89 | 12.21 | 9.84 | 10.31 | 9.62 | 10.70 | 10.13 |
| NO | 9.26 | 4.53 | 12.82 | 10.06 | 10.79 | 9.93 | 10.85 | 10.57 |
| $O_2$ | 12.30 | 7.29 | 15.95 | 13.24 | 13.69 | 12.86 | 14.04 | 13.40 |
| $H_2O_2$ | 11.70 | 6.50 | 14.19 | 11.57 | 11.64 | 10.87 | 12.27 | 11.43 |
| $F_2$ | 15.70 | 9.66 | 18.96 | 16.92 | 16.09 | 15.14 | 16.75 | 15.81 |
| $CO_2$ | 13.78 | 9.30 | 15.29 | 14.72 | 14.08 | 13.13 | 14.75 | 13.86 |
| $Na_2$ | 4.89 | 3.19 | 5.11 | 5.17 | 5.13 | 4.97 | 4.87 | 4.75 |
| $Si_2$ | 7.90 | 5.13 | 9.00 | 8.32 | 8.52 | 8.18 | 8.69 | 8.32 |
| $P_2$ | 10.62 | 7.15 | 10.27 | 10.78 | 10.61 | 9.94 | 10.91 | 10.42 |
| $S_2$ | 9.55 | 5.88 | 11.16 | 9.90 | 10.03 | 9.65 | 11.18 | 9.87 |
| $Cl_2$ | 11.49 | 7.45 | 13.14 | 11.49 | 11.78 | 11.28 | 12.78 | 11.01 |
| NaCl | 9.80 | 5.32 | 10.19 | 9.66 | 9.68 | 8.62 | 10.00 | 8.98 |
| SiO | 11.49 | 7.61 | 12.77 | 11.48 | 11.75 | 11.09 | 12.01 | 11.58 |
| CS | 11.33 | 7.45 | 12.86 | 11.33 | 11.63 | 10.97 | 11.71 | 11.42 |
| SO | 11.29 | 6.02 | 12.63 | 10.84 | 11.23 | 10.71 | 11.45 | 11.01 |
| ClO | 11.01 | 6.47 | 13.73 | 11.56 | 11.76 | 11.11 | 12.09 | 11.31 |
| ClF | 12.77 | 8.05 | 14.48 | 13.30 | 13.20 | 12.59 | 13.21 | 12.57 |
| $Si_2H_6$ | 10.53 | 7.36 | 12.28 | 10.46 | 10.92 | 10.58 | 10.97 | 10.68 |
| $CH_3Cl$ | 11.29 | 7.15 | 12.72 | 11.76 | 11.65 | 10.97 | 11.79 | 11.15 |
| $CH_3SH$ | 9.44 | 5.66 | 10.80 | 9.43 | 9.75 | 9.22 | 9.91 | 9.50 |
| HOCl | 11.12 | 6.81 | 13.18 | 11.46 | 11.47 | 10.92 | 12.00 | 11.08 |
| $SO_2$ | 12.50 | 8.30 | 14.45 | 12.50 | 12.86 | 12.20 | 13.41 | 12.68 |

Table II. Tabulated ionization energies (in eV) for all molecules of the G2-1 set and for all functionals discussed in the paper having LDA as base functional, and being minimized on the space of complex wavefunctions.

| | exp | PBE | PZ | KI | KIPZ | $K_0$ |
|---|---|---|---|---|---|---|
| LiH | 7.90 | 4.35 | 8.62 | 6.97 | 6.82 | 6.64 |
| BeH | 8.21 | 4.74 | 8.67 | 8.43 | 8.35 | 8.60 |
| CH | 10.64 | 5.96 | 11.80 | 10.84 | 10.60 | 10.42 |
| $CH_2$_s3B1d | 10.40 | 5.80 | 11.21 | 10.90 | 10.27 | 10.08 |
| $CH_3$ | 9.84 | 5.51 | 10.27 | 9.88 | 9.57 | 9.42 |
| $CH_4$ | 13.60 | 9.43 | 15.63 | 14.05 | 13.95 | 13.68 |
| NH | 13.49 | 7.62 | 14.52 | 13.31 | 12.87 | 12.43 |
| $NH_2$ | 12.00 | 7.16 | 13.66 | 12.02 | 11.78 | 11.25 |
| $NH_3$ | 10.82 | 6.17 | 12.18 | 10.96 | 10.58 | 10.05 |
| OH | 13.02 | 7.37 | 14.97 | 13.34 | 12.76 | 12.10 |
| $H_2O$ | 12.62 | 7.24 | 14.26 | 12.76 | 12.25 | 11.56 |
| HF | 16.12 | 9.61 | 17.81 | 16.28 | 15.63 | 14.75 |
| $SiH_2$_s1A1d | 8.92 | 5.83 | 10.12 | 9.66 | 9.34 | 9.36 |
| $SiH_3$ | 8.74 | 5.35 | 9.67 | 9.15 | 8.91 | 8.94 |
| $SiH_4$ | 12.30 | 8.52 | 13.97 | 12.35 | 12.45 | 12.36 |
| $PH_2$ | 9.82 | 6.05 | 10.61 | 10.41 | 9.82 | 9.67 |
| $PH_3$ | 10.95 | 6.63 | 11.23 | 10.37 | 10.36 | 10.15 |
| $SH_2$ | 10.50 | 6.28 | 11.12 | 10.44 | 10.26 | 9.91 |
| HCl | 12.74 | 8.02 | 13.40 | 12.61 | 12.52 | 12.06 |
| $Li_2$ | 5.11 | 3.22 | 5.34 | 5.12 | 5.02 | 4.47 |
| LiF | 11.30 | 6.11 | 13.19 | 11.76 | 11.14 | 10.18 |
| $C_2H_2$ | 11.49 | 7.16 | 12.10 | 11.26 | 11.10 | 10.66 |
| $C_2H_4$ | 11.49 | 6.75 | 11.80 | 10.51 | 10.49 | 10.04 |
| $C_2H_6$ | 12.00 | 8.12 | 14.27 | 12.19 | 12.01 | 12.08 |
| CN | 13.60 | 9.60 | 15.05 | 14.08 | 13.69 | 13.06 |
| HCN | 13.61 | 8.94 | 14.30 | 13.37 | 13.32 | 12.83 |
| CO | 14.01 | 9.07 | 15.24 | 14.00 | 13.82 | 13.49 |
| HCO | 9.31 | 5.09 | 11.82 | 9.81 | 9.80 | 9.64 |
| $H_2CO$ | 10.88 | 6.25 | 13.27 | 11.81 | 10.47 | 10.09 |
| $CH_3OH$ | 10.96 | 6.29 | 13.14 | 11.18 | 10.48 | 10.06 |
| $N_2$ | 15.58 | 10.23 | 17.18 | 15.95 | 15.41 | 15.14 |
| $N_2H_4$ | 8.98 | 5.78 | 11.95 | 10.69 | 9.85 | 9.42 |
| NO | 9.26 | 4.55 | 12.38 | 10.67 | 9.94 | 9.88 |
| $O_2$ | 12.30 | 7.21 | 15.58 | 13.20 | 12.60 | 12.24 |
| $H_2O_2$ | 11.70 | 6.36 | 13.81 | 12.04 | 10.98 | 10.65 |
| $F_2$ | 15.70 | 9.46 | 18.32 | 15.83 | 15.19 | 14.80 |
| $CO_2$ | 13.78 | 9.06 | 15.35 | 14.20 | 13.02 | 12.81 |
| $Na_2$ | 4.89 | 3.22 | 5.05 | 5.10 | 4.98 | 3.99 |
| $Si_2$ | 7.90 | 5.03 | 8.72 | 8.37 | 8.05 | 7.91 |
| $P_2$ | 10.62 | 7.02 | 10.66 | 10.43 | 10.25 | 9.93 |
| $S_2$ | 9.55 | 5.89 | 11.03 | 9.66 | 9.61 | 9.34 |
| $Cl_2$ | 11.49 | 7.34 | 12.86 | 11.75 | 11.22 | 11.07 |
| NaCl | 9.80 | 5.24 | 9.93 | 9.44 | 9.02 | 8.38 |
| SiO | 11.49 | 7.48 | 12.50 | 11.74 | 11.14 | 10.89 |
| CS | 11.33 | 7.39 | 13.03 | 10.92 | 10.91 | 10.54 |
| SO | 11.29 | 6.07 | 12.39 | 10.59 | 10.63 | 10.52 |
| ClO | 11.01 | 6.42 | 13.11 | 11.05 | 11.12 | 11.02 |
| ClF | 12.77 | 7.92 | 13.98 | 12.27 | 12.63 | 12.43 |
| $Si_2H_6$ | 10.53 | 7.30 | 11.99 | 9.97 | 10.51 | 10.42 |
| $CH_3Cl$ | 11.29 | 7.06 | 12.51 | 11.45 | 11.06 | 10.75 |
| $CH_3SH$ | 9.44 | 5.57 | 10.51 | 10.33 | 9.23 | 8.98 |
| HOCl | 11.12 | 6.69 | 12.81 | 11.53 | 10.86 | 10.65 |
| $SO_2$ | 12.50 | 8.10 | 14.48 | 12.12 | 12.12 | 11.93 |

Table III. Tabulated ionization energies (in eV) for all molecules of the G2-1 set and for all functionals discussed in this paper having PBE as base functional, and being minimized in the space of real wavefunctions.

| | exp | PBE | PZ | KI | KIPZ | $K_0$ |
|---|---|---|---|---|---|---|
| LiH | 7.90 | 4.35 | 8.62 | 6.97 | 6.82 | 6.64 |
| BeH | 8.21 | 4.74 | 8.67 | 8.69 | 8.35 | 8.60 |
| CH | 10.64 | 5.97 | 11.43 | 11.08 | 10.65 | 10.42 |
| $CH_2$_s3B1d | 10.40 | 5.80 | 10.74 | 10.78 | 10.30 | 10.02 |
| $CH_3$ | 9.84 | 5.51 | 10.14 | 10.26 | 9.69 | 9.37 |
| $CH_4$ | 13.60 | 9.43 | 15.61 | 14.12 | 13.95 | 13.68 |
| NH | 13.49 | 7.63 | 14.03 | 13.53 | 12.85 | 12.42 |
| $NH_2$ | 12.00 | 7.16 | 12.90 | 12.29 | 11.73 | 11.20 |
| $NH_3$ | 10.82 | 6.17 | 11.78 | 11.01 | 10.55 | 10.03 |
| OH | 13.02 | 7.37 | 14.21 | 13.30 | 12.85 | 12.08 |
| $H_2O$ | 12.62 | 7.24 | 13.76 | 12.83 | 12.31 | 11.67 |
| HF | 16.12 | 9.61 | 17.24 | 16.29 | 15.62 | 14.63 |
| $SiH_2$_s1A1d | 8.92 | 5.82 | 10.12 | 9.41 | 9.30 | 9.26 |
| $SiH_3$ | 8.74 | 5.35 | 9.67 | 8.93 | 8.91 | 8.94 |
| $SiH_4$ | 12.30 | 8.52 | 13.97 | 12.11 | 12.45 | 12.36 |
| $PH_2$ | 9.82 | 6.05 | 10.42 | 10.23 | 9.79 | 9.67 |
| $PH_3$ | 10.95 | 6.64 | 11.23 | 10.60 | 10.36 | 10.15 |
| $SH_2$ | 10.50 | 6.28 | 10.81 | 10.35 | 10.20 | 9.90 |
| HCl | 12.74 | 8.02 | 12.85 | 12.86 | 12.42 | 12.03 |
| $Li_2$ | 5.11 | 3.22 | 5.34 | 5.12 | 5.02 | 4.47 |
| LiF | 11.30 | 6.11 | 13.12 | 11.93 | 11.28 | 10.12 |
| $C_2H_2$ | 11.49 | 7.16 | 11.16 | 11.36 | 10.84 | 10.37 |
| $C_2H_4$ | 11.49 | 6.75 | 11.45 | 10.67 | 10.54 | 9.94 |
| $C_2H_6$ | 12.00 | 8.12 | 14.25 | 11.98 | 11.93 | 12.00 |
| CN | 13.60 | 9.60 | 14.33 | 14.20 | 13.61 | 12.85 |
| HCN | 13.61 | 8.94 | 13.49 | 13.42 | 13.16 | 12.60 |
| CO | 14.01 | 9.07 | 15.27 | 13.93 | 13.77 | 13.50 |
| HCO | 9.31 | 5.09 | 11.57 | 9.61 | 9.71 | 9.79 |
| $H_2CO$ | 10.88 | 6.25 | 12.75 | 10.68 | 10.40 | 10.05 |
| $CH_3OH$ | 10.96 | 6.29 | 12.33 | 11.87 | 10.38 | 9.81 |
| $N_2$ | 15.58 | 10.23 | 16.40 | 15.40 | 15.25 | 15.03 |
| $N_2H_4$ | 8.98 | 5.78 | 11.40 | 9.96 | 9.69 | 9.42 |
| NO | 9.26 | 4.55 | 12.08 | 10.15 | 10.15 | 9.82 |
| $O_2$ | 12.30 | 7.21 | 14.80 | 14.23 | 13.04 | 12.61 |
| $H_2O_2$ | 11.70 | 6.36 | 12.91 | 11.93 | 10.87 | 10.57 |
| $F_2$ | 15.70 | 9.46 | 17.58 | 16.41 | 15.26 | 14.71 |
| $CO_2$ | 13.78 | 9.06 | 14.75 | 14.88 | 13.43 | 12.88 |
| $Na_2$ | 4.89 | 3.22 | 5.05 | 5.10 | 4.98 | 3.99 |
| $Si_2$ | 7.90 | 5.03 | 8.63 | 8.14 | 8.10 | 7.90 |
| $P_2$ | 10.62 | 7.02 | 10.04 | 10.52 | 10.08 | 9.73 |
| $S_2$ | 9.55 | 5.89 | 10.62 | 9.84 | 9.64 | 9.58 |
| $Cl_2$ | 11.49 | 7.34 | 12.44 | 11.35 | 11.27 | 11.06 |
| NaCl | 9.80 | 5.24 | 9.82 | 9.37 | 9.05 | 8.33 |
| SiO | 11.49 | 7.48 | 12.33 | 11.23 | 11.06 | 10.77 |
| CS | 11.33 | 7.39 | 12.52 | 11.03 | 11.06 | 10.64 |
| SO | 11.29 | 6.07 | 12.20 | 10.76 | 10.81 | 10.67 |
| ClO | 11.01 | 6.42 | 13.05 | 11.42 | 11.06 | 10.86 |
| ClF | 12.77 | 7.92 | 13.64 | 13.04 | 12.56 | 12.33 |
| $Si_2H_6$ | 10.53 | 7.30 | 11.99 | 10.30 | 10.51 | 10.42 |
| $CH_3Cl$ | 11.29 | 7.06 | 12.04 | 11.50 | 11.11 | 10.72 |
| $CH_3SH$ | 9.44 | 5.57 | 10.22 | 9.21 | 9.19 | 8.98 |
| HOCl | 11.12 | 6.69 | 12.23 | 11.72 | 10.74 | 10.63 |
| $SO_2$ | 12.50 | 8.10 | 13.95 | 12.67 | 12.09 | 11.76 |

Table IV. Tabulated ionization energies (in eV) for all molecules of the G2-1 set and for all functionals discussed in this paper having PBE as base functional, and being minimized in the space of complex wavefunctions.
